# Supplementary material for: Four Years of FAccT: A Reflexive, Mixed-Methods Analysis of Research Contributions, Shortcomings, and Future Prospects
Source: arXiv:2206.06738 source file (2022-06-14)
Supplement: Supplementary file 1 [file FAccT_perspectives_appendix.pdf]

# Introduction

This questionnaire aims to solicit your views on FAccT (Fairness, Accountability, and Transparency) scholarship, in particular, publications that have appeared in the ACM FAccT conference. Your answers will contribute to a research project studying research trends, gaps, and opportunities in the field.

The survey contains 3 main sections:
- Views on FAccT scholarship and recommendations for future improvements
- The intellectual merit and broader impact of several FAccT *research topics*
- The broader impact of FAccT scholarship in several *application domains*

The main questionnaire will be followed with an (optional) set of questions about your background and affiliation with the FAccT community.

To be mindful of your time, we have made all of the questions optional to respond to, but we would appreciate your input on as many of them as you believe you are qualified to respond to. Please do NOT respond to questions that you do not feel sufficiently informed/qualified to answer. At any point during the questionnaire, you can skip to the last section and submit the form (even if incomplete).

## Views and Recommendations

This section seeks to elicit your opinion about several facets of FAccT scholarship, including
- Its most significant critiques
- Recommendations for future improvements

1. To what extent has the FAccT conference exposed its members to insights and ideas from other disciplines?

*Mark only one oval.*

| | 1 | 2 | 3 | 4 | 5 | |
|---|---|---|---|---|---|---|
| Very low exposure | ◯ | ◯ | ◯ | ◯ | ◯ | Very high exposure |

2. Reviewers of the FAccT conference come from various disciplines and backgrounds. In your experience, how has this impact the quality of the conference's peer review?

*Mark only one oval.*

| | 1 | 2 | 3 | 4 | 5 | |
|---|---|---|---|---|---|---|
| Has severely impeded it | ◯ | ◯ | ◯ | ◯ | ◯ | Has significantly improved it |

3. Many FAccT publications use publicly available datasets as part of their analysis. What is your overall assessment of the quali of these datasets for obtaining significant insights?

*Mark only one oval.*

| | 1 | 2 | 3 | 4 | 5 | |
|---|---|---|---|---|---|---|
| Very Low Quality | ◯ | ◯ | ◯ | ◯ | ◯ | Very High Quality |

4. Are there any moral or social values (sufficiently distinct from Fairness, Accountability, and Transparency) that you believe FAccT scholarship should address in near future?

5. What do you consider to be the most important criticisms of FAccT scholarship to date?

6. How do you believe the FAccT conference can address the above issues and limitations in the near future?

7. Any additional thoughts about FAccT?

## Research Topics

In the questions that follow, you will be asked to rate the "intellectual merit" and "broader impact" of previous FAccT publications addressing several research topics, as well as how much FAccT scholarship should prioritize each topic.

The topics in this section are extracted from the "areas/tracks" of prior ACM FAccT conferences. (They are not necessarily mutually exclusive or exhaustive).

We have adopted the terms "intellectual merit" and "broader impact" from NSF (National Science Foundation), which defines:

- "Intellectual merit" as the contribution to advancement of knowledge and understanding. (Criteria include sound rationale and reasoning motivating the research, presenting creative, original, or potentially transformative concepts/approaches, well-organized execution of the research, positive scholarly impact within or outside the field).

- "Broader impacts" as benefits to society and contributions to the achievement of specific, desired societal outcomes. (Examples include empowering disadvantaged or marginalized individuals and communities; improving equity of access to opportunities; improving literacy and engagement of researchers, practitioners and the public).

### Scoring Instructions

For each of the following topics, please score with 1 (indicating very low) up to 5 (indicating very high):

- The intellectual merit of *previous* FAccT publications on the topic.

- The broader impact of *previous* FAccT publications on the topic.

- Your assessment of whether *future* FAccT scholarship should prioritize this topic.

8. Algorithm Development

(e.g. fairness-enhancing algorithms; interpretable and explainable models)

*Mark only one oval per row.*

| | 1 (very low) | 2 | 3 | 4 | 5 (very high) |
|---|---|---|---|---|---|
| Intellectual Merit | ⬭ | ⬭ | ⬭ | ⬭ | ⬭ |
| Broader Impact | ⬭ | ⬭ | ⬭ | ⬭ | ⬭ |
| Should FAccT Prioritize this Topic? | ⬭ | ⬭ | ⬭ | ⬭ | ⬭ |

9. Community-based Approaches and Human Factors

(e.g. participatory algorithm design; community designed and maintained systems; activism-driven technological change, human-computer interaction; humans-ir the-loop; information visualization; UX design)

*Mark only one oval per row.*

| | 1 (very low) | 2 | 3 | 4 | 5 (very high) |
|---|---|---|---|---|---|
| Intellectual Merit | | | | | |
| Broader Impact | | | | | |
| Should FAccT Prioritize this Topic? | | | | | |

10. Data and Algorithm Evaluation

(e.g. metrics; audits; data collection and curation)

*Mark only one oval per row.*

| | 1 (very low) | 2 | 3 | 4 | 5 (very high) |
|---|---|---|---|---|---|
| Intellectual Merit | | | | | |
| Broader Impact | | | | | |
| Should FAccT Prioritize this Topic? | | | | | |

11. Law, Policy, and Governance

(e.g. data protection; non-discrimination; fair procedures; human rights; oversight mechanisms; organizational governance; codes of ethics; models from historically marginalized perspectives)

*Mark only one oval per row.*

| | 1 (very low) | 2 | 3 | 4 | 5 (very high) |
|---|---|---|---|---|---|
| Intellectual Merit | | | | | |
| Broader Impact | | | | | |
| Should FAccT Prioritize this Topic? | | | | | |

12. Philosophy, Historical and Cultural Analysis

(e.g. philosophical foundations of machine learning; values in scientific inquiry; social epistemology; moral, legal and political philosophy of data and AI; Interrogating foundational concepts; Bridging critical concepts across fields)

*Mark only one oval per row.*

| | 1 (very low) | 2 | 3 | 4 | 5 (very high) |
|---|---|---|---|---|---|
| Intellectual Merit | | | | | |
| Broader Impact | | | | | |
| Should FAccT Prioritize this Topic? | | | | | |

13. Please briefly describe how you believe "impact" *should* be defined for FAccT scholarship.

## Application Domains

The following section is concerned with several real-world, socially high-stakes domains in which algorithmic, data-driven tools have been utilized.

For each of the following domains, we would like you to score (with 1=very low up to 5=very high) the broader impact of previous FAccT publications for the domain's practices

A reminder that we have adopted the term "broader impact" from NSF (National Science Foundation), which defines "Broader impacts" as benefits to society and contributions to the achievement of specific, desired societal outcomes. (Examples include empowering disadvantagec or marginalized individuals and communities; improving equity of access to opportunities; improving literacy and engagement of researchers, practitioners and the public).

14. FAccT's Broader Impact on Domains

*Mark only one oval per row.*

| | Unfamiliar | 1 (very low) | 2 | 3 | 4 | 5 (very high) |
|---|---|---|---|---|---|---|
| Criminal Justice System | | | | | | |
| Education | | | | | | |
| Healthcare/Medical | | | | | | |
| Hiring/Employment | | | | | | |
| Internet Advertising | | | | | | |
| Social Media | | | | | | |
| Social Services | | | | | | |

## Information About You

Please tell us about yourself to the extent that you are comfortable. Remember that the questionnaire is anonymous. (All categorical alternatives have been ordered alphabetically).

15. Which of the following areas of scholarship best describes your expertise?

*Check all that apply.*

- [ ] HSA (Humanities, Social Sciences and the Arts)
- [ ] STEM (Science, Technology, Engineering, Mathematics)

Other: [ ] ______

16. If you have played any formal role in the FAccT conference (including the main conference, as well as its workshops, tutorial CRAFT sessions), select all that apply.

*Check all that apply.*

- [ ] Attendee
- [ ] Author
- [ ] Organizing Committee Member
- [ ] Reviewer

Other: [ ] ______

17. How many years have you been affiliated with the FAccT conference?

*Mark only one oval.*

| | 0 | 1 | 2 | 3 | 4 | 5 | |
|---|---|---|---|---|---|---|---|
| 0 year of involvement | ◯ | ◯ | ◯ | ◯ | ◯ | ◯ | 5 years of involvement |

18. Which of the following best describes your political views? (Please pick the closest approximation if none is exactly right).

*Mark only one oval.*

- ◯ Conservative
- ◯ Liberal
- ◯ Libertarian
- ◯ Other: ______________________

19. Do you belong to a marginalized/disadvantaged group or community?

*Mark only one oval.*

- ◯ No
- ◯ Yes

20. If you would like to communicate anything else about yourself with us, please do so here.

21. Thank you so much for your participation. If you have any feedback for us about the questionnaire, please leave your comments here, or email the PI.

## Interested in participating in one-on-one, open-ended interviews?

Please contact the PI (hheidari@cmu.edu) if you are interested in participating in a longer interview with the research team to provide us with your detailed thoughts assessments of FAccT.

This content is neither created nor endorsed by Google.

Google Forms
